# Supplementary material for: Selective Radiance in Super-Wavelength Atomic Arrays
Source: arXiv:2402.06439 ancillary file (2024-02-09)
Supplement: Supplementary file 1 [file Supplementary_Material.pdf]

# Supplementary Material:
# Selective Radiance in Super-Wavelength Atomic Arrays

Charlie-Ray Mann,[1] Francesco Andreoli,[1] Vladimir Protsenko,[2] Zala Lenarčič,[2] and Darrick E. Chang[1,3]

[1]*ICFO-Institut de Ciencies Fotoniques, The Barcelona Institute of Science and Technology, 08860 Castelldefels (Barcelona), Spain.*
[2]*Jožef Stefan Institute, SI-1000 Ljubljana, Slovenia.*
[3]*ICREA-Institució Catalana de Recerca i Estudis Avançats, 08015 Barcelona, Spain.*

## CONTENTS

I. Projection into a detection mode – general ensemble 1

II. Linear response – general ensemble 3

III. Projection into a detection mode – idealized model 3

IV. Linear response – idealized model 4

V. Super-wavelength mirror configurations 4

References 5

## I. PROJECTION INTO A DETECTION MODE – GENERAL ENSEMBLE

In this section we provide more details on the mode projection formalism that we use for calculating the observables in an arbitrary detection mode. We note that a conceptually similar discussion appears in ref.[1], although we believe the following exposition is more transparent and fixes some errors mistakes there. First, let's assume the atoms are located at $\mathbf{r}_i$ and the entire ensemble is confined to some finite region $\mathbb{V}$ centred at the origin. The field scattered by the ensemble is given by

$$\hat{\mathbf{E}}^+_{\text{scat}}(\mathbf{r},t_r) = \frac{\hbar\Gamma_0}{|\wp|}\sum_i \bar{\bar{\mathbf{G}}}(\mathbf{r}-\mathbf{r}_i,\omega_0)\cdot\mathbf{e}_\wp\,\hat{\sigma}^i_{ge}(t)\,, \tag{S1}$$

which is evaluated at an advanced time $t_r = t + r/c$ with respect to the atomic operators (we neglect time-retardation within the ensemble). Typically, the collection optics and detectors are located far from the ensemble $k_0 r \gg 1$ where only the (power-carrying) far-field component is relevant.

We can introduce a set of monochromatic, outgoing field modes $\{\boldsymbol{\mathcal{O}}_m(\mathbf{r})\}$ which satisfy the homogeneous vector Helmholtz equation in the source-free region outside $\mathbb{V}$ and Sommerfield's radiation boundary condition

$$\nabla\times(\nabla\times\boldsymbol{\mathcal{O}}_m) - k_0^2\boldsymbol{\mathcal{O}}_m = 0\,, \qquad \lim_{r\to\infty} r\,[\hat{\mathbf{r}}\times(\nabla\times\boldsymbol{\mathcal{O}}_m) - \mathrm{i}k_0\boldsymbol{\mathcal{O}}_m] = 0\,, \tag{S2}$$

where $\hat{\mathbf{r}} = \mathbf{r}/r$ is the radial unit vector. In the far-field limit these outgoing modes can be conveniently expressed as

$$\boldsymbol{\mathcal{O}}_m(\mathbf{r}) \sim -2\pi\mathrm{i}\frac{\mathrm{e}^{\mathrm{i}k_0 r}}{k_0 r}\mathbf{F}_m(\theta,\phi)\,, \tag{S3}$$

where $\mathbf{F}_m = F^\phi_m\hat{\boldsymbol{\phi}} + F^\theta_m\hat{\boldsymbol{\theta}}$ is a transverse vector field (no radial component) which we will refer to as the far-field radiation pattern (it can also be related to the angular spectrum representation [2]). Here, $\hat{\boldsymbol{\phi}}$ and $\hat{\boldsymbol{\theta}}$ are the usual spherical unit vectors and $F^\phi_m$ and $F^\theta_m$ are the corresponding components. For our purposes, it is useful to define the inner product based on the notion of power orthogonality where the different modes carry power independently through an arbitrary surface $S$ that encloses the ensemble (see Fig. 1a). The relevant inner product is therefore

$$(\boldsymbol{\mathcal{O}}_m|\boldsymbol{\mathcal{O}}_n) = -\mathrm{i}\frac{k_0}{(2\pi)^2}\oiint_S [\boldsymbol{\mathcal{O}}^*_m\times(\nabla\times\boldsymbol{\mathcal{O}}_n)]\cdot\mathrm{d}\mathbf{A} = \oiint_{S_\infty}\mathrm{d}\Omega\,\mathbf{F}^*_m\cdot\mathbf{F}_n\,, \tag{S4}$$

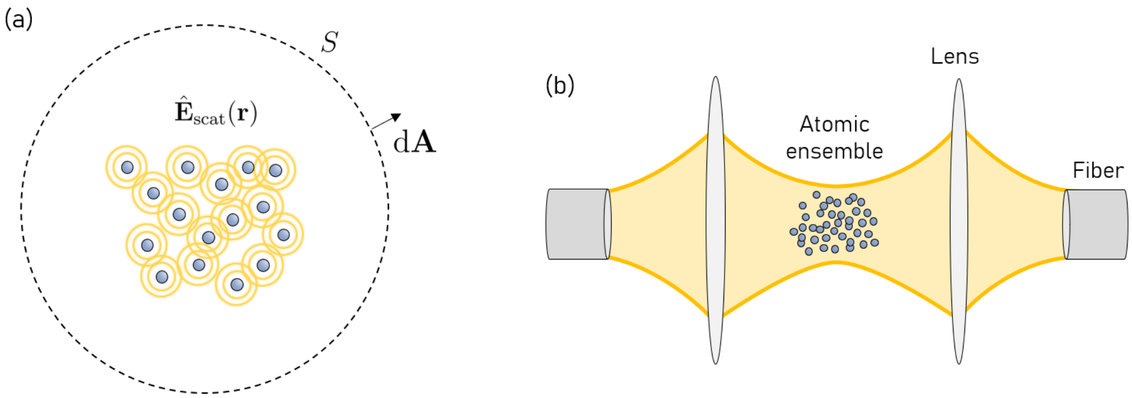


FIG. 1. (a) Schematic of an atomic ensemble which scatters photons into outgoing modes that carry power through a closed surface $S$. (b) Typical experimental set-up where the collection optics are set-up to efficiently capture photons emitted into a well-defined spatial mode.

where $\mathrm{d}\mathbf{A}$ is the infinitesimal area element oriented normal to the surface $S$ in the outward direction. In the second line we have used the freedom to define a spherical surface at infinity $S_\infty$, so that we can invoke the far-field expressions in Eq. (S3). We have also used the shorthand notation $\oiint \mathrm{d}\Omega = \int_0^\pi \mathrm{d}\theta \sin\theta \int_0^{2\pi} \mathrm{d}\phi$ to indicate the integral over the full solid angle. This expression tells us that the inner product corresponds to the spatial overlap of the far-field radiation patterns.

We can expand the propagating component of the scattered field in terms of these outgoing modes

$$\hat{\mathbf{E}}^+_{\rm scat}(\mathbf{r}, t_r) \sim \mathcal{N} \sum_m \boldsymbol{\mathcal{O}}_m(\mathbf{r}) \hat{a}_m(t) \tag{S5}$$

where we assume the modes are orthonormal $(\boldsymbol{\mathcal{O}}_m|\boldsymbol{\mathcal{O}}_n) = \delta_{mn}$. We choose the prefactor factor $\mathcal{N} = (3\hbar^2\Gamma_0/8\pi|\wp|^2)^{1/2}$ so that $\langle \hat{a}^\dagger_m(t)\hat{a}_m(t)\rangle$ corresponds to the instantaneous rate of photons scattered into the outgoing mode $\boldsymbol{\mathcal{O}}_m$. Moreover, the total scattering rate is simply given an independent sum $n_{\rm scat}(t) = \sum_m \langle \hat{a}^\dagger_m(t)\hat{a}_m(t)\rangle$.

We now suppose the experiment is set up to efficiently capture photons that are emitted into a given detection mode $\boldsymbol{\mathcal{O}}_{\rm det}$ (see Fig. 1b), and the associated quantum operator is given by $\hat{a}_{\rm det,scat} = \mathcal{N}^{-1}(\boldsymbol{\mathcal{O}}_{\rm det}|\hat{\mathbf{E}}_{\rm scat})$. To calculate this overlap we first need the far-field limit of the free space Green's function which reads

$$\bar{\bar{\mathbf{G}}}(\mathbf{r}, \mathbf{r}_i) \sim -2\pi \mathrm{i} \frac{\mathrm{e}^{\mathrm{i}k_0 r}}{k_0 r} \bar{\bar{\mathbf{F}}}_G \quad , \quad \bar{\bar{\mathbf{F}}}_G = \frac{3\mathrm{i}}{8\pi} \mathrm{e}^{-\mathrm{i}k_0 \hat{\mathbf{r}}\cdot\mathbf{r}_i} \left(\bar{\bar{\mathbf{I}}} - \hat{\mathbf{r}} \otimes \hat{\mathbf{r}}\right). \tag{S6}$$

Then, by noting that the term inside the bracket is just the unit dyad in the space of transverse fields, it is simple to show that the overlap with the Green's function is

$$(\boldsymbol{\mathcal{O}}_{\rm det}|\bar{\bar{\mathbf{G}}}(\mathbf{r}, \mathbf{r}_i)) = \oiint \mathrm{d}\Omega\, \mathbf{F}^*_{\rm det} \cdot \bar{\bar{\mathbf{F}}}_G = \frac{3\mathrm{i}}{8\pi} \boldsymbol{\mathcal{E}}^*_{\rm det}(\mathbf{r}_i), \tag{S7}$$

which results in the following expression for the quantum operator

$$\hat{a}_{\rm det,scat}(t) = \mathrm{i}\sqrt{\frac{3\Gamma_0}{8\pi}} \sum_i \boldsymbol{\mathcal{E}}^*_{\rm det}(\mathbf{r}_i) \cdot \mathbf{e}_\wp\, \hat{\sigma}^i_{ge}(t). \tag{S8}$$

Here we have defined the associated homogeneous detection mode

$$\boldsymbol{\mathcal{E}}_{\rm det}(\mathbf{r}) = \oiint \mathrm{d}\Omega\, \mathbf{F}_{\rm det}(\theta, \phi) \mathrm{e}^{\mathrm{i}k_0(\sin\theta\cos\phi x + \sin\theta\sin\phi y + \cos\theta z)}, \tag{S9}$$

which is a solution to the homogeneous Helmholtz equation in the entire space. Note that this is neither an outgoing or an incoming wave, but we can still calculate overlaps and normalize the modes according to the inner product $(\boldsymbol{\mathcal{E}}_m|\boldsymbol{\mathcal{E}}_n) = \oiint \mathrm{d}\Omega\, \mathbf{F}^*_m \cdot \mathbf{F}_n$. Finally, to arrive at Eq. (4) in the main text, we have to include the contribution of the input field $\hat{\mathbf{E}}^+_{\rm in}(\mathbf{r}, t_r) = \mathcal{N}\boldsymbol{\mathcal{E}}_{\rm in}(\mathbf{r})\hat{a}_{\rm in}(t)$, where the input mode $\boldsymbol{\mathcal{E}}_{\rm in}(\mathbf{r})$ is normalized so that $\langle \hat{a}^\dagger_{\rm in}\hat{a}_{\rm in}\rangle$ corresponds to the rate of incident photons. The corresponding detection mode operator is given by

$$\hat{a}_{\rm det,in}(t) = \frac{1}{\mathcal{N}} (\boldsymbol{\mathcal{E}}_{\rm det}|\boldsymbol{\mathcal{E}}_{\rm in})\hat{a}_{\rm in}(t). \tag{S10}$$

## II. LINEAR RESPONSE – GENERAL ENSEMBLE

In this section we derive the linear reflection coefficient for a finite atomic ensemble subjected to a continuous-wave input field at normal incidence. For the spatial input mode we consider a Gaussian beam propagating along the $z$ direction which, in the paraxial approximation, reads

$$\boldsymbol{\mathcal{E}}_{\rm in}(\mathbf{r}) \simeq \mathcal{E}_0 \frac{w}{w(z)} \mathrm{e}^{-\frac{\rho^2}{w(z)^2}} \mathrm{e}^{\mathrm{i}[(k_0 z - \varphi(z) + k_0\rho^2/2R(z))]} \boldsymbol{\epsilon}_{\rm in} \,. \tag{S11}$$

The normalization constant $\mathcal{E}_0 \simeq \sqrt{8\pi}/k_0 w$ is chosen such that $(\boldsymbol{\mathcal{E}}_{\rm in}|\boldsymbol{\mathcal{E}}_{\rm in}) = 1$, and the polarization is chosen to match the atomic transition such that $\mathbf{e}_\wp^* \cdot \boldsymbol{\epsilon}_{\rm in} = 1$. We have also introduced the usual quantities for a Gaussian beam $w(z) = w(1+\zeta^2)^{1/2}$, $R(z) = z(1+\zeta^2)$ and $\varphi(z) = \arctan(\zeta)$ where the reduced coordinate is $\zeta = z/z_{\rm R}$ with $z_{\rm R} = k_0 w^2/2$.

If we assume that the input field is weak enough so that the dynamics are effectively restricted to the single excitation manifold, then we can use the following ansatz for the general state

$$|\psi(t)\rangle = \big[c_g(t) + \sum_i c_i(t)\hat{\sigma}_{eg}^i\big]|g\rangle^{\otimes N} \,. \tag{S12}$$

In the low saturation regime ($c_g(t) \approx 1$) the equation of motion for the excited state amplitudes read

$$\dot{c}_i(t) = \mathrm{i}\Delta c_i(t) + \mathrm{i}\Gamma_0 \sum_j G_{ij} c_j(t) + \mathrm{i}\Omega_i \,, \tag{S13}$$

and the steady state solution ($\dot{c}_i = 0$) can be written in matrix form as

$$\vec{c} = -\langle \hat{a}_{\rm in}\rangle \sqrt{\frac{3}{8\pi\Gamma_0}} \bar{\bar{\Lambda}} \cdot \vec{\mathcal{E}} \,. \tag{S14}$$

Here we have defined the vector of excited state amplitudes $\vec{c} = (c_1, c_2, \ldots, c_N)^{\rm T}$, the input vector $\vec{\mathcal{E}} = (\mathcal{E}_1, \mathcal{E}_2, \ldots, \mathcal{E}_N)^T$ with $\mathcal{E}_i = \mathbf{e}_\wp^* \cdot \boldsymbol{\mathcal{E}}_{\rm in}(\mathbf{r}_i)$, and the linear response matrix $\bar{\bar{\Lambda}}$ whose elements are given by $(\bar{\bar{\Lambda}}^{-1})_{ij} = (\Delta/\Gamma_0)\delta_{ij} + G_{ij}$.

From this one can calculate the reflection coefficient $r = \langle \hat{a}_{\rm det}\rangle / \langle \hat{a}_{\rm in}\rangle$ for any arbitrary detection mode. Here, we will focus on the specular reflection, where the homogeneous detection mode is taken to be the same as the Gaussian input mode but propagating in the opposite direction. This means $\mathcal{E}_i = \mathbf{e}_\wp^* \cdot \boldsymbol{\mathcal{E}}_{\rm in}(\mathbf{r}_i) = \mathbf{e}_\wp \cdot \boldsymbol{\mathcal{E}}^*_{\rm det}(\mathbf{r}_i)$, and thus the reflection coefficient reads

$$r = -\frac{3\mathrm{i}}{8\pi} \vec{\mathcal{E}} \cdot \bar{\bar{\Lambda}} \cdot \vec{\mathcal{E}} \,, \tag{S15}$$

as given in the main text.

## III. PROJECTION INTO A DETECTION MODE – IDEALIZED MODEL

In this section we describe how to adapt the projection formalism for the idealized model with $N \to \infty$ and a plane wave input. Since we have discrete translational symmetry in the $xy$-plane, the array can only scatter light into a discrete set of plane wave modes (i.e., diffraction orders). However, there is a subtlety when applying the projection formalism outlined in Sec. I because plane waves do not reside in the physical Hilbert space of normalizable modes (i.e., plane waves carry infinite power).

Our aim is to calculate the reflectance which is just the ratio of the scattered power (into the detection mode) to the input power, and therefore the absolute power is not important. Pragmatically, to overcome these formal subtleties we can just renormalize the inner product in Eq. (S4) by dividing by the number of unit cells in the array $N \to \infty$. With this, the quantum operator associated with a plane wave detection mode is

$$\hat{a}_{\rm det}(t) = \hat{a}_{\rm det,in}(t) + \frac{\mathrm{i}}{N}\sqrt{\frac{3\Gamma_0}{8\pi}} \sum_{i\alpha} \boldsymbol{\mathcal{E}}^*_{\rm det}(\mathbf{r}_{i\alpha}) \cdot \mathbf{e}_\wp \, \hat{\sigma}_{ge}^{i\alpha}(t) \,, \tag{S16}$$

where $\langle \hat{a}^\dagger_{\rm det}(t)\hat{a}_{\rm det}(t)\rangle$ now corresponds to the rate of photons per unit cell entering the detection mode. Note that to normalize the plane wave modes according to the modified inner product it is convenient to deform the infinite spherical surface into two infinite parallel planes that enclose the multi-layer array.

## IV. LINEAR RESPONSE – IDEALIZED MODEL

In this section we derive the reflection coefficient for a multi-layer array in the idealized limit $N \to \infty$. The normalized plane wave input mode can be written as

$$\boldsymbol{\mathcal{E}}_{\text{in}}(\mathbf{r}) = \sqrt{\frac{4\pi}{3}\frac{\Gamma_{00}}{\Gamma_0}}\mathrm{e}^{\mathrm{i}k_0 z}\boldsymbol{\epsilon}_{\text{in}}\,, \tag{S17}$$

which can only excite the $\mathbf{q} = \mathbf{0}$ spin waves in each layer. Therefore, we can use the following ansatz for the general state

$$|\psi(t)\rangle = \big[c_g(t) + \sum_\alpha c_\alpha(t)\hat{S}^\dagger_\alpha\big]|g\rangle^{\otimes NM}\,. \tag{S18}$$

Using the effective Hamiltonian given by Eq. (7) in the main text one finds that the excited state amplitudes obey the following equation of motion in the low saturation limit

$$\dot{c}_\alpha(t) = \mathrm{i}(\Delta - J)c_\alpha(t) + \mathrm{i}\Gamma_{00}\sum_\beta \mathcal{G}_{\alpha\beta}c_\beta(t) + \mathrm{i}\sqrt{N}\Omega_\alpha\,. \tag{S19}$$

Here, the layer-dependent Rabi frequency is $\Omega_\alpha = \wp^* \cdot \mathbf{E}^+_{\text{in}}(z_\alpha)/\hbar$, and the inter-layer matrix elements are given by Eq. (8) in the main text. As before, we are interested in the steady-state solution which can be expressed in matrix form as

$$\vec{c} = -\langle\hat{a}_{\text{in}}\rangle\sqrt{\frac{NM}{2\Gamma_{00}}}\bar{\bar{\Lambda}}\cdot\vec{U}\,, \tag{S20}$$

where we have defined the vector of layer amplitudes $\vec{c} = (c_1, c_2, \dots, c_M)^{\mathrm{T}}$, the normalized input vector $\vec{U} = (U_1, U_2, \dots, U_M)^T$ with $U_\alpha = M^{-1/2}\mathrm{e}^{\mathrm{i}k_0 z_\alpha}$, and the linear response matrix $\bar{\bar{\Lambda}}$ whose elements are given by $(\bar{\bar{\Lambda}}^{-1})_{\alpha\beta} = (\Delta - J)/\Gamma_{00}\delta_{\alpha\beta} + \mathcal{G}_{\alpha\beta}$.

From here one can calculate the reflection coefficient $r = \langle\hat{a}_{\text{det}}\rangle/\langle\hat{a}_{\text{in}}\rangle$ for any diffraction order using the modified projection formalism. Here, we focus on the specular reflection and take the homogeneous detection mode to be the same as the input plane wave mode but propagating in the opposite direction. The corresponding reflection coefficient is

$$r = -\frac{\mathrm{i}M}{2}\vec{U}\cdot\bar{\bar{\Lambda}}\cdot\vec{U} = \frac{\mathrm{i}M\Gamma_{00}}{2}\sum_\xi \frac{(\vec{U}\cdot\vec{v}_\xi)^2}{-\Delta + J - \Gamma_{00}\lambda_\xi}\,, \tag{S21}$$

where $\lambda_\xi$ and $\vec{v}_\xi$ are the set of $M$ eigenvalues and eigenvectors of the matrix $\mathcal{G}_{\alpha\beta}$, rspectively, which satisfy the relations $\vec{v}_\xi\cdot\vec{v}_{\xi'} = \delta_{\xi\xi'}$ and $\sum_\xi \vec{v}_\xi\otimes\vec{v}_\xi = \bar{\bar{I}}$. For a monolayer ($M = 1$) there is only one eigenstate with eigenvalue $\lambda = \mathrm{i}/2$ and thus the reflection coefficient has a simple Lorentzian form which can be expressed as

$$r = \frac{\mathrm{i}\Gamma_{\text{det}}/2}{-\Delta + J - \mathrm{i}(\Gamma_{\text{det}} + \Gamma_{\text{diff}})/2}\,, \tag{S22}$$

with $\Gamma_{\text{det}} = \Gamma_{00}$ and $\Gamma_{\text{diff}} = \sum_{mn\neq 00}\Gamma_{mn}$, which is the same as Eq. (5) in the main text.

## V. SUPER-WAVELENGTH MIRROR CONFIGURATIONS

In this section we provide some additional details about the critical super-wavelength mirror configurations with $d = \ell\lambda_0/2$. When $Q \in \mathbb{N}_{\text{even}}$ the matrix elements read

$$\mathcal{G}_{\alpha\beta} = \frac{\mathrm{i}}{2\Gamma_{00}}\begin{cases}\Gamma_{00} + \Gamma' & \text{for} \quad \alpha+\beta\in\mathbb{N}_{\text{even}}\\ (-1)^\ell(\Gamma_{00} + \Gamma') & \text{for} \quad \alpha+\beta\in\mathbb{N}_{\text{odd}}\end{cases} \tag{S23}$$

where we have used the shorthand notation $\Gamma' = \sum_{mn\neq 00}\Gamma_{mn}$. Evidently, this is a rank-1 matrix as there is only one linearly-independent row/column. In constrast, for $Q \in \mathbb{N}_{\text{odd}}$ the matrix elements are

$$\mathcal{G}_{\alpha\beta} = \frac{\mathrm{i}}{2\Gamma_{00}}\begin{cases}\Gamma_{00} + \Gamma' & \text{for} \quad \alpha+\beta\in\mathbb{N}_{\text{even}}\\ (-1)^\ell(\Gamma_{00} - \Gamma') & \text{for} \quad \alpha+\beta\in\mathbb{N}_{\text{odd}}\end{cases} \tag{S24}$$

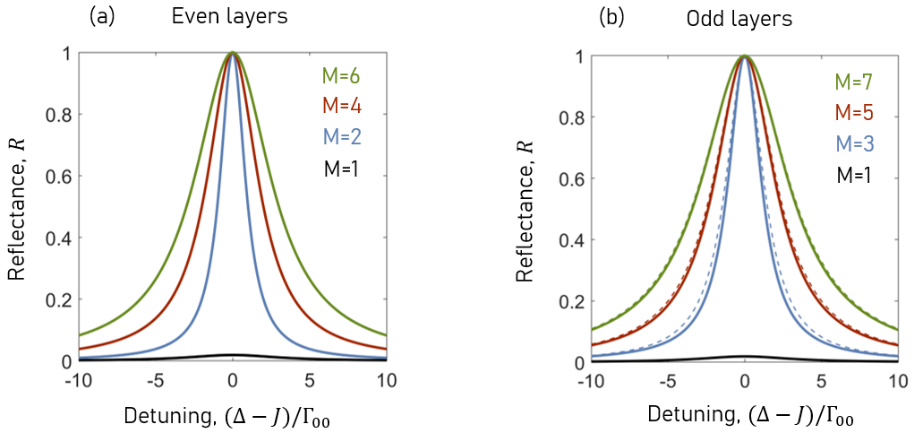


FIG. 2. (a) Reflectance spectrum for a triangular super-wavelength mirror configuration with an even number of layers and a plane wave input at normal incidence ($d = 2\lambda_0$, $a = 1.746$). For comparison, we also plot the reflectance for a monolayer. (b) Same plot but now for an odd number of layers, and the dotted lines indicate a Lorentzian lineshape of width $M\Gamma_{00}$.

which is a rank-2 matrix because there are now two linearly-independent rows/columns.

As discussed in the main text, for an even number of layers there is a bright state $|B_2\rangle$ that selectively radiates into the specular detection mode at an enhanced rate $\Gamma_{\rm det} = M\Gamma_{00}$, while the emission into the diffraction orders is completely suppressed $\Gamma_{\rm diff} = 0$. Using Eq. (S21) we plot the reflectance spectrum in Supplementary Fig. 2a for a triangular super-wavelength mirror configuration with an even number of layers and a plane wave input at normal incidence. For concreteness, we choose the mirror configuration $(a, d) = (2\lambda_0, 1.746\lambda_0)$, but we note that the spectrum is the same for any other mirror configuration within this idealized model. The response is a Lorentzian of width $M\Gamma_{00}$ due to the single state response, and the plane wave is perfectly reflected on resonance due to the selective radiance.

In Supplementary Fig. 2b we plot the reflectance spectrum for an odd number of layers and, for comparison, we also indicate a Lorentzian lineshape of width $M\Gamma_{00}$ with dotted lines. The physics is more subtle here because the two bright eigenstates do not exhibit perfect selective radiance into the specular mode and diffraction orders, respectively. As a result, both states contribute to the response, although the dominant contribution is still from $|B_2\rangle$, and one still obtains perfect reflection on resonance. As one would expect, the slight difference between even and odd layers diminishes rapidly as the number of layers increase and the reflectance spectrum becomes indistinguishable from a Lorentzian.

[1] M. Manzoni, M. Moreno-Cardoner, A. Asenjo-Garcia, J. V. Porto, A. V. Gorshkov, and D. Chang, New journal of physics **20**, 083048 (2018).
[2] L. Novotny and B. Hecht, *Principles of nano-optics* (Cambridge university press, 2012).
